# Supplementary material for: Giant anomalous Hall effect in quasi-two-dimensional layered antiferromagnet Co$_{1/3}$NbS$_2$
Source: arXiv:2004.08896 ancillary file (2020-04-23)
Supplement: Supplementary file 1 [file Co1_3NbS2_SI.pdf]

**Supplemental Material**  
**Giant anomalous Hall effect in quasi-two-dimensional layered**  
**antiferromagnet  $\text{Co}_{1/3}\text{NbS}_2$**

Giulia Tenasini,<sup>1,2</sup> Edoardo Martino,<sup>3</sup> Nicolas Ubrig,<sup>1,2</sup> Nirmal J.  
Ghimire,<sup>4,5,6</sup> Helmuth Berger,<sup>3</sup> Oksana Zaharko,<sup>7</sup> Fengcheng Wu,<sup>6,8</sup> J.  
F. Mitchell,<sup>6</sup> Ivar Martin,<sup>6</sup> László Forró,<sup>3</sup> and Alberto F. Morpurgo<sup>1,2,\*</sup>

<sup>1</sup>*Department of Quantum Matter Physics, University of Geneva,  
24 Quai Ernest Ansermet, CH-1211 Geneva, Switzerland*

<sup>2</sup>*Group of Applied Physics, University of Geneva, 24  
Quai Ernest Ansermet, CH-1211 Geneva, Switzerland*

<sup>3</sup>*Laboratory of Physics of Complex Matter, École polytechnique  
Fédérale de Lausanne, 1015 Lausanne, Switzerland*

<sup>4</sup>*Department of Physics and Astronomy, George  
Mason University, Fairfax, Virginia 22030, USA*

<sup>5</sup>*Quantum Materials Center, George Mason University, Fairfax, Virginia 22030, USA.*

<sup>6</sup>*Materials Science Division, Argonne National Laboratory, Lemont, Illinois 60439, USA*

<sup>7</sup>*Laboratory for Neutron Scattering and Imaging,  
Paul Scherrer Institut, Villigen PSI, Switzerland*

<sup>8</sup>*Condensed Matter Theory Center and Joint Quantum Institute, Department  
of Physics, University of Maryland, College Park, Maryland 20742, USA*

---

\* [Alberto.morpurgo@unige.ch](mailto:Alberto.morpurgo@unige.ch)

## S1. DEVICE FABRICATION

In this section we describe in more details the sample fabrication for the two different types of nano-structured devices investigated in the main manuscript.

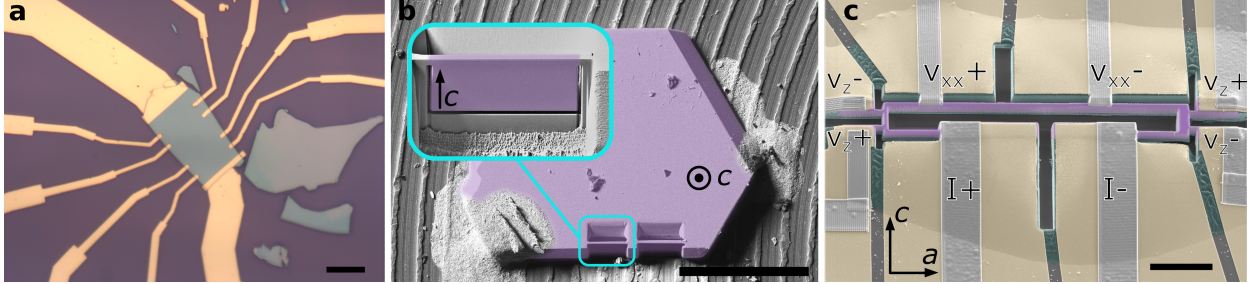

FIG. S1. **a**, Optical micrograph of a representative Co<sub>1/3</sub>NbS<sub>2</sub> exfoliated crystal with metal contacts in a Hall-bar configuration (the scale bar represents 10  $\mu\text{m}$ ). **b**, Electron microscopy (SEM) false color image of a single crystal (purple) from which rectangular lamellas are created by focused ion beam (FIB) milling (the scale bar represents 500  $\mu\text{m}$ ). **c**, SEM false color image of a device sculpted with FIB, starting from a lamella like the ones shown in **b**. The single crystal (in purple) is cut as a continuous current path between the two current leads (I). Three sets of voltage probes enable to measure the resistivity along the NbS<sub>2</sub> planes ( $V_{xx}$ ) and perpendicular ( $V_z$ ). The gold films to connect the device to the electrodes are colored in yellow, and the Pt-strips deposited using the FIB in grey (the scale bar represents 10  $\mu\text{m}$ ).

**Exfoliated crystal devices.** Co<sub>1/3</sub>NbS<sub>2</sub> crystals are mechanically exfoliated from bulk material using a common adhesive tape and transferred onto conventional Si/SiO<sub>2</sub> substrates, i.e., highly p-doped silicon covered with a 285 nm layer of thermally grown silicon oxide. The crystal thickness –which is not easily identified by optical contrast on SiO<sub>2</sub> as the material is metallic and few tens of nanometer thick– is determined measuring the height profiles with atomic force microscopy (AFM). Source and drain electrodes, as well as the Hall probes are realized by conventional nano-fabrication techniques, based on electron beam lithography, evaporation of Ti/Au films, and lift-off. Optical micrographs of representative devices are shown in Fig. S1a or in Fig. 1e in the main manuscript. The devices are finally mounted on a chip carrier and wire bonded.

**Focused Ion Beam (FIB) devices.** The FIB microfabrication to prepare samples

for resistivity anisotropy measurements, is conducted using a FEI Helios G3, dual beam (SEM/FIB) microscope [S1]. Starting from a carefully pre-characterized single crystal, a rectangular lamella is extracted by ions milling perpendicular to the crystal growth surface (along the c-axis), as shown in Fig. S1b. Before extraction, the lamella surfaces are polished by grazing angle milling at a significantly lower beam current, in order to remove the extent of the amorphous layer produced by the interaction with the ions. Subsequently the lamella is transferred onto a sapphire substrate, and fixed by a drop of epoxy glue. When the epoxy is cured, a gold film is deposited by radio frequency (RF) sputtering over the entire sample area. Platinum strips are deposited using the FIB to ensure stronger adhesion and stability of the voltage and current leads on the microstructure. The device is patterned into its final shape (Fig. S1c), and the individual electrical contacts are made by etching through the previously deposited gold layer [S1]. Gold wires are attached by silver epoxy to create the final connections to the experimental set-up.

## S2. ADDITIONAL DATA FOR THE DEVICE SHOWING SIGNATURE OF STRUCTURAL DOMAIN SWITCHING

In the main manuscript we discuss data from measurements on a device showing an unexpected jump in the anomalous Hall resistivity,  $\rho_{xy}^A$ , as function of temperature, at about 17 K (see Fig. 4a). This peculiar behavior is attributed to the presence of a domain wall in the antiferromagnetic state, most likely due to the existence of a stacking fault along the NbS<sub>2</sub> planes of the considered crystal. Here, we show in detail the magnetic field dependence of the Hall resistivity,  $\rho_{xy}$ , (Fig. S2a) and of the anomalous Hall resistivity (Fig. S2b) for this device. As also mentioned in the main text,  $\rho_{xy}^A$  exhibits an anomalous hysteresis comprising two loops when the magnetic field is cycled from  $-14$  T to  $+14$  T and back; this is indeed what is shown by the orange curve measured at 27 K. Upon cooling down the device, the coercive field increases such rapidly that the second transition cannot be observed anymore at temperatures as high as 25 K (red curve). From Fig. S2b we extract the  $H = 0$  value of  $\rho_{xy}^A$  at different temperatures and plot them in Fig. 4a in the main text (yellow diamonds) together with the temperature dependence of  $\rho_{xy}^A$  after field-cooling. For the high-field state we extract the value of  $\rho_{xy}^A$  at  $\mu_0 H = 14$  T and plot the data points as light-blue diamonds

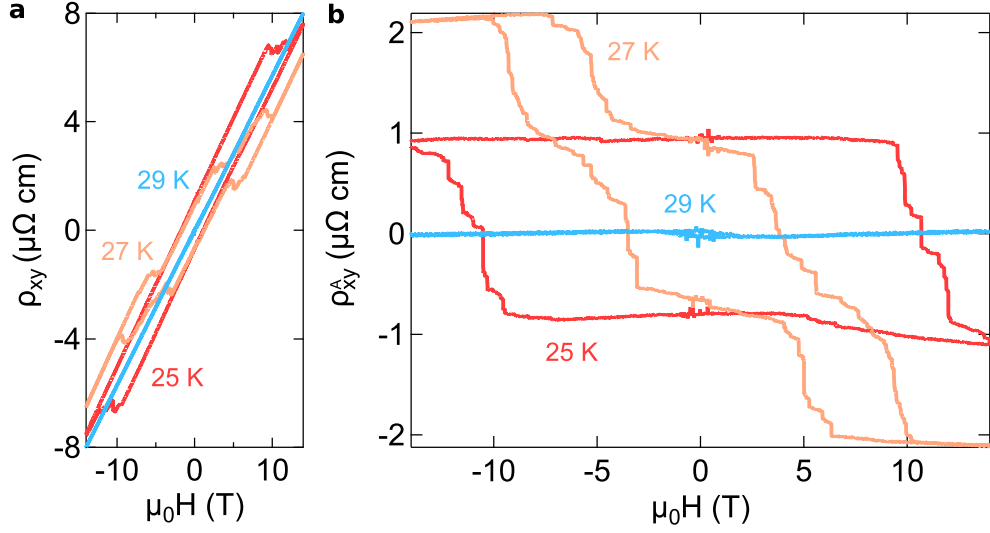

FIG. S2. Magnetic field dependence of (a) Hall resistivity  $\rho_{xy}$  and (b) anomalous Hall resistivity  $\rho_{xy}^A$  measured at selected temperatures below  $T_N$  in the same device whose data are shown in Fig. 4.  $\rho_{xy}^A$  in b is obtained by subtracting from the data in a the ordinary linear Hall effect contribution. At 27 K (orange curve) an anomalous hysteresis loop comprising two distinct parts is observed. Upon cooling down the sample, the coercive field rapidly increases and at  $T$  as high as 25 K (red curve) the second jump in the hysteresis loop cannot be detected anymore within the magnetic field range accessible in our experimental set-up ( $\pm 14$  T).

in Fig. 4a in the main text.

---

[S1] P. J. Moll, [Annual Review of Condensed Matter Physics](#) **9**, 147 (2018).
